# Supplementary material for: Dynamics of soliton crystals in optical microresonators
Source: arXiv:1903.07122 ancillary file (2019-09-03)
Supplement: Supplementary file 1 [file SI_1um_v4.pdf]

# Supplementary Information - Dynamics of soliton crystals in optical microresonators

Maxim Karpov, Martin H. P. Pfeiffer, Tobias J. Kippenberg
École Polytechnique Fédérale de Lausanne (EPFL), CH-1015 Lausanne, Switzerland
(Dated: March 17, 2019)

## Simulations

In order to investigate soliton crystals numerically we use coupled-mode-based approach of the simple LLE model with the dispersion limited to the second-order term, and omitted Raman and thermal effects:

$$\frac{\partial A(\phi,t)}{\partial t}=\sqrt{\frac{\kappa\eta P_{\mathrm{in}}}{\hbar\omega_0}}-\left(\frac{\kappa}{2}+i(\omega_0-\omega_p)\right)A(\phi,t)-i\frac{D_2}{2}\frac{\partial^2 A(\phi,t)}{\partial\phi^2}+ig|A(\phi,t)|^2A(\phi,t) \tag{1}$$

Here $A(\phi,t)$ is the slowly varying intracavity field amplitude defined on the co-rotating angular coordinate $\phi=\varphi-D_1t$ with the regular polar angle $\varphi$ and free spectral range, FSR $=D_1/2\pi$. The angular frequencies of the pumped resonance and the CW driving laser are denoted as $\omega_0$ and $\omega_p$ correspondingly. Total cavity losses are described with the photon escape rate $\kappa=\kappa_0+\kappa_{ex}$, which includes the internal losses $\kappa_0$ and the coupling to the bus waveguide $\kappa_{ex}$. The ratio $\kappa_{ex}/\kappa$ is denoted as $\eta$. The nonlinearity is described via $g=\hbar\omega_0^2cn_2/n_0^2V_{\mathrm{eff}}$ giving the Kerr frequency shift per photon, where $n_2$ is the nonlinear refractive index, $n_0$ is the effective group refractive index and $V_{\mathrm{eff}}$ is the effective optical mode volume. The dispersion is introduced through the second-order group velocity dispersion (GVD) term $D_2=-\frac{\beta_2cD_1^2}{n_0}$. In order to enable the formation of soliton crystals the set of coupled modes was perturbed by introducing an additional detuning change for a certain mode with a mode number $\xi$, such that the detuning value for such a comb line is $\delta\omega_\xi=\omega_p-\omega_\xi=\omega_p-(\omega_0+D_1\xi+\Delta)$, where $\Delta$ accounts for the mode shifting due to the impact of the spectrally localized avoided modal crossing (AMX). The simulations were performed with 512 modes. We used the measured parameters of the real device from our experiment, which includes: FSR = 95.4 GHz, $D_2/2\pi=1.3$ MHz, $\kappa/2\pi=200$ MHz, $\eta=1/2$, $\omega_0/2\pi=193.46$ THz. The parameters of the perturbation introduced for the soliton crystals are: $\xi=15$, $\Delta/2\pi=130$ MHz. The position of the modal crossing $\xi=15$ was choosen in order to enable the formation of a perfect soliton crystal consisting of 15 DKS pulses. The "strength" of the modal crossing $\Delta/2\pi$ was set to to satisfy two conditions: (i) it should be large enough to enable the crystallization of the intracavity field in a PSC state with given parameters of the microresonator system; (ii) The perturbation it introduces to the system is small and does not affect the formation of multiple-soliton states (e.g. by shortening the DKS steps or introducing significant inter-mode breathing).

For the map simulations, the above-described system was initialized with a perfect soliton crystal solution at various values of pump-cavity detuning ($\omega_p-\omega_0$) and pump power ($P_{\mathrm{in}}$), and was propagating for about 5000 roundtrips to reach the stable state. The obtained stable states were classified in several regions: stable PSC state, breathing PSC state, spatiotemporal chaos, transient chaos, modulation instability (MI) and homogeneous (CW) solutions, which were marked with corresponding colours on the stability chart (see Supplementary Fig.1(a)). In order to demonstrate the behaviour of the system in each of them, we explicitly plot the evolution of the intracavity intensity during about 25000 roundtrips, which was excited with a perfect soliton crystal solution at six different fixed detunings and the same pump power $P_{\mathrm{in}}=1$W (see Supplementary Fig.1(b)).

## Spatiotemporal chaos and transient chaos regions

We would like to focus on and illustrate here the system behavior in the two important regions of our study - spatiotemporal chaos (STC) and transient chaos (TC). First we note that both of them lie within the bistability boundaries of the system, meaning that in both regions the system has stable homogeneous solution (lower-branch solution), which we will also refer to as the "CW solution". We start by considering the region of spatiotemporal chaos (STC), colored with grey in the stability chart - here the system experiences chaotic spatial and temporal oscillations of the intracavity waveform, which can be observed in plot 2 of Fig.1(b). The system is initialized with a perfect soliton crystal solution and immediately demonstrates a transition to chaotic behaviour, which continues for more than 20000 roundtrips with no sign of degradation or evident changes in its dynamics.

The second region is that of transient chaos, where the system experiences a long (in comparison to the photon escape rate) chaotic decay to a certain stable (however, not necessary steady-state) solution. The region is coloured with yellow in Fig.1(a), and the intracavity intensity evolution in this region is shown in plot 3 of Fig.1(b). The system is initiated with a soliton crystal solution, and in this particular example for about two thousand of roundtrips

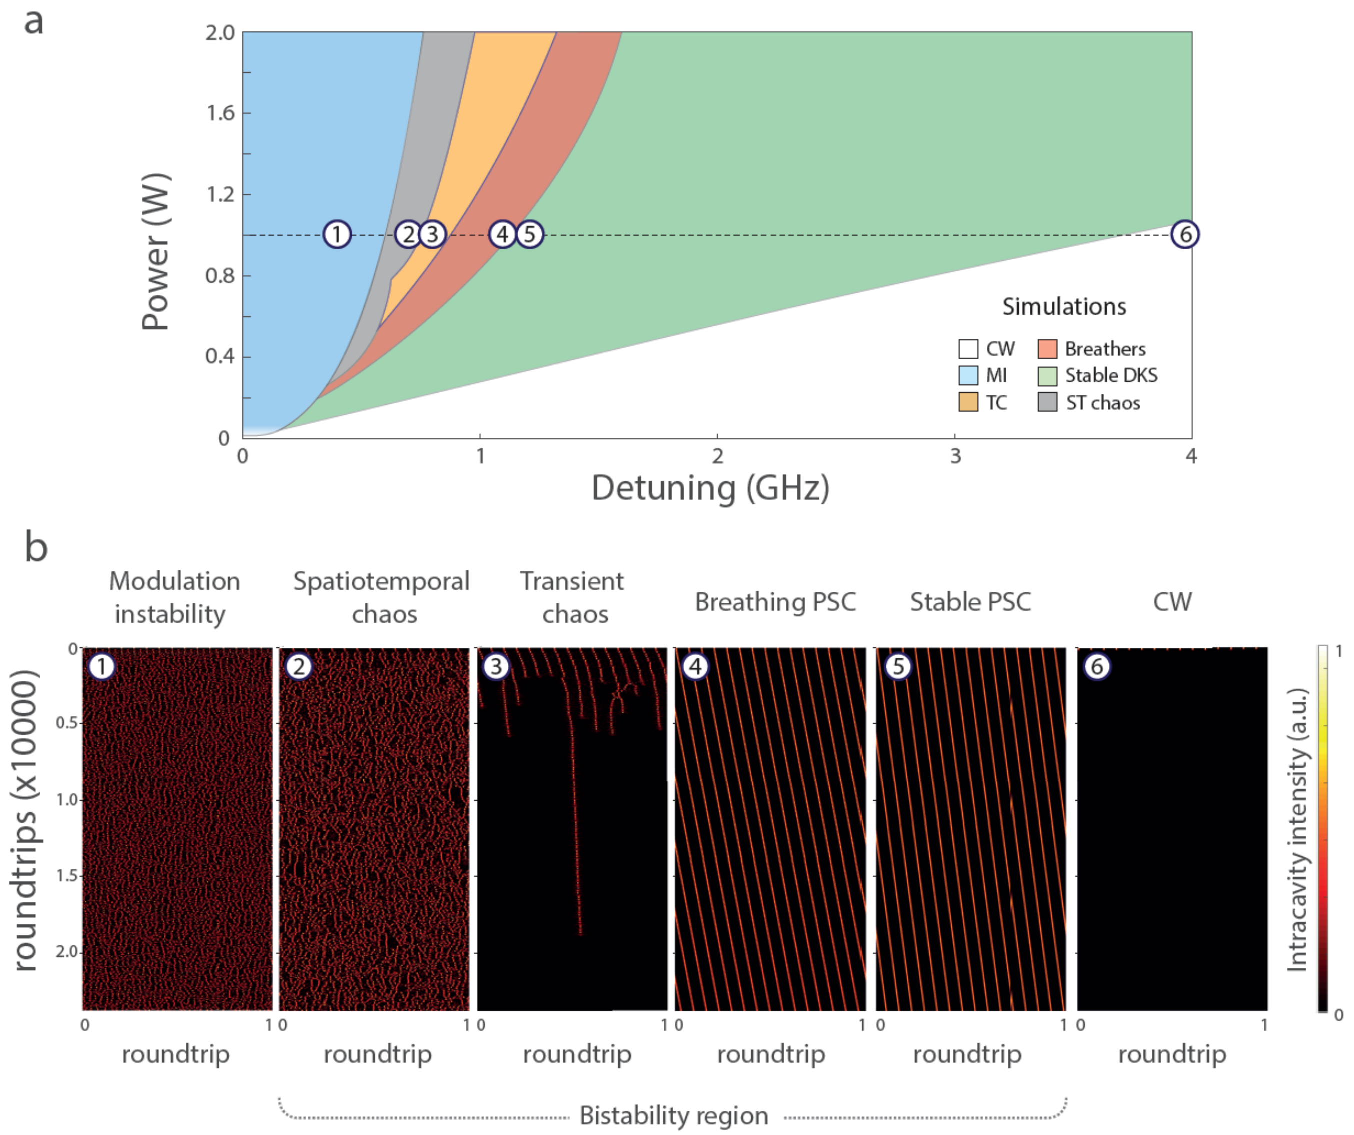


Supplementary Figure 1. **Stability chart simulations for perfect soliton crystals** (a) Simulated stability chart of the Lugiato-Lefever equation augmented with one AMX crossing located at $\xi = 15$; The coloured areas indicate different stability regions of the PSC states: stable PSC - green, breathing PSC - red, modulation instability - blue, spatiotemporal chaos (STC) - grey, transient chaos (TC) - yellow, CW solutions - white. Numbered circles indicate six simulations made in different stability regimes, which evolutions are plotted in (b). (b) Simulations of the intracavity intensity evolution at fixed pump-cavity detuning and pump power in six different stability regions marked in (a). All simulations are initialized with a PSC solution and were propagated for about 25000 roundtrips (from top to bottom of each graph).

it maintains its spatial order, while having temporally chaotic behaviour. After this, the intracavity waveform start to spontaneously lose DKS pulses. They may decay on their own or first experience interactions with adjacent soliton. Such process continues until the last pulse decays (around 18000 roundtrips for our simulation) and the intracavity waveform ultimately becomes only the CW solution. We note that depending on the seed, the general pattern of the spontaneous decay from an initial PSC state to a final state may change significantly, but it always has two main features in this TC region that we observed in our simulations: first, the decay of the intracavity field mostly happens *pulse-wise*, which is in contrast to decay of the state outside of the bistability region (see e.g. plot 6 in Fig.1(b); second, the final state of the system will have a stable attractor, which might be a CW or non-stationary multiple-soliton state.

We would like to point out some subtle differences between the stability chart we obtained for soliton crystal state (Fig.1(a)) and the stability chart, obtained for single-soliton states in earlier work for similar driven Kerr-

nonlinear system [1]. Apart from general similarity, one can note that the region of transient chaos that was found in the simulations by Leo *et al.* starts at around $f = 5$, while in our simulations its bottom extends down to $f \sim 4$. The difference here is in the following, for $f > 5$, the system in both cases (single soliton state and PSC state) reveals transient chaotic behavior and always decays to a homogeneous solution (CW solution). While for $4 < f < 5$ the evolution of the system initiated with a single soliton state and PSC state will differ. In the first case the intracavity waveform will maintain its spatially inhomogeneous structure (DKS pulse) with periodic or possibly chaotic oscillations. In the second case, a PSC state will not be maintained and will relax to a multiple-soliton state with lower number of DKS. This behaviour means that in the second case the system also undergoes transient chaotic processes, where the final state is not a homogeneous solution but a low-number-soliton state. Since our map is plotted with respect to a PSC state it's natural to classify the latest scenario as *transient chaos*.

An interesting consequence of this behaviour can be also observed in experiments. As can be seen from the results shown in Fig.3(b) of the main manuscript, the number of available switchings between DKS states depends on *pump power*. In particular, when the system just overcomes $P_{\mathrm{sw}}$, it can be switched only once - from a perfect soliton crystal state to a soliton crystal state with a defect. All other attempts of backward tuning at the same pump power will just transfer the system into a modulation instability state without access to other DKS states. However, at higher pump powers more switchings become available, and the system can reach multiple-soliton states with low soliton number. Eventually, only above $f \sim 5$ can the system be switched up to a single soliton state and further to the CW solution, before it enters modulation instability state. Figure 2 illustrates two experiments, where we performed backward tuning from a PSC state with the pump power below $P_{\mathrm{sw}}$ (Fig.2(a)) or just above it (Fig.2(b)). In the first case the system switches directly from a PSC state (green shaded area) to the blue-detuned modulation instability (unshaded). In the secon case, the system first experiences one switch to a soliton crystal state with a defect (light green shading) and then also falls in to MI. Rising the pump power further can lead to the case when almost all-number soliton states become available and we can reach a single soliton state, as shown in Fig.3(c) of the main manuscript.

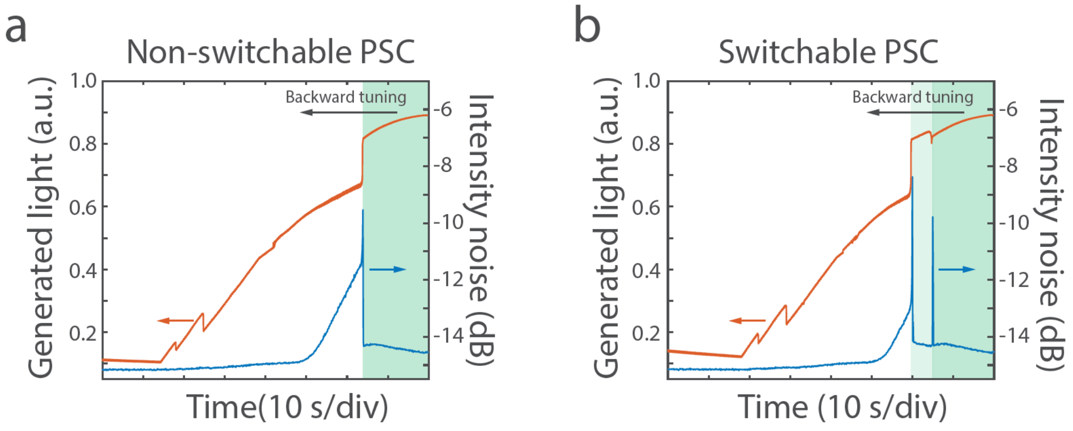


Supplementary Figure 2. **Characterization of dissipative Kerr soliton states in hybridized modes.** (a, b) Evolution of the generated light power (red) and total intensity noise (blue) measured during the backward tuning procedure from a PSC state for two pump powers: below $P_{\mathrm{sw}}$(a) and just above it (b). Soliton states are shaded green, modulation instability region is unshaded. transition to MI can also be traced by the significantly increased total intensity noise. The switching transition in (b) can be also observed by a characteristic spike attributed to the onset of breathing before switching.

We also compare here our stability chart for the PSC state to the one simulated in the recent paper by Wang *et al* [2] for soliton crystal states. There are two key differences with our work. The first difference is in the existence range of SC states, which in the case of Wang *et al.* was constrained to the small area below the breathing region. In contrast, in our stability chart the existence range for soliton crystals spans behind the chaotic regions and has no upper boundaries in pump power and pump detuning (similar to the stability of the single soliton states [1, 3]). The second difference is in the absence of chaotic regions (STC and TC) for soliton crystal states generated by Wang *et al.* In our opinion, the differences originate from the way of simulating the stability chart, which in the case of Wang *et al.* was based on the dynamic simulations of the intracavity waveform evolution during pump frequency sweeps (continuously changing the detuning from the blue-detuned to the red-detuned) at different fixed pump powers. While being relatively fast, such approach can mask the stable soliton crystal solutions behind the chaotic regimes, because, as shown in our manuscript, they prohibit the formation of the soliton crystals in the forward tuning regime, used by Wang *et al.* for simulating the stability chart. We rely on our results, because we experimentally demonstrated

the existence of the PSC states within the boundaries obtained in our simulations spanning well beyond the region suggested by Wang *et al.* Furthermore, for the simulations we followed an already established approach, which was used and experimentally confirmed for single soliton states in optical fiber cavities [1]. Besides, it also allows clear identification of the chaotic regimes, which as shown in the main text of our manuscript, determine the dynamics of soliton crystal states.

Nevertheless, the formation of soliton crystal states presented in the paper by Wang *et al*[2], as well as the switching of DKS states presented by the same group [4] provide a good example of the previous experimental observations, which are fully explained using the theoretical framework developed in our main manuscript regarding the impact of the STC and TC regions on the dynamics of soliton crystal states. Both works employed the same microresonator platform of thermally-tunable high-index doped silica glass (hydex) microring resonator with almost identical parameters. The critical difference between two works was in the **pump power**, which has been increased by more than a factor of 2 (from 30.5 dBm [2] to $>$ 34.5 dBm [4]) and completely changed the system dynamics and resulted in different observations. At lower pump power[2], the authors observed the formation of defective soliton crystal states (similar to [5]) and also reported the observation of PSC-like state with small irregularities resulted in the appearance of weak native-comb modes together with the supermodes in the optical spectrum of the state. All of the demonstrated states were accessed with thermal tuning, and reported to be unswitchable. In contrast, the second paper[4] reported on the observation of DKS switching in the same system, but operating at much higher pump power. Unlike the first paper, the initial state, generated by Lu *et al.* via sweeping the temperature of the microresonator, did not have clear supermodes typical for the SC states. It can be rather interpreted as having multiple defects, breaking the pulses regularity and inhibiting the supermode formation. Comparing the power dependence of the results observed in both papers, we can make a direct link to our manuscript, and explain both observations through the impact of TC and STC regimes. At lower pump power [2] the system operates at the bottom of the STC region for a given microresonator, which has resulted in the stochastic formation of PSC or soliton crystal states with very low number of defects. Since the TC region is located at higher pump powers, the switching was not observed. In contrast, at higher pump power[4] the system is heavily impacted by both chaotic regions. This enables the switching, but prevents the formation of low-defect-number soliton states, which explains why the initial state generated at higher pump power did not have well-defined supermodes and its optical spectrum had the typical shape for multiple-soliton states rather than a PSC.

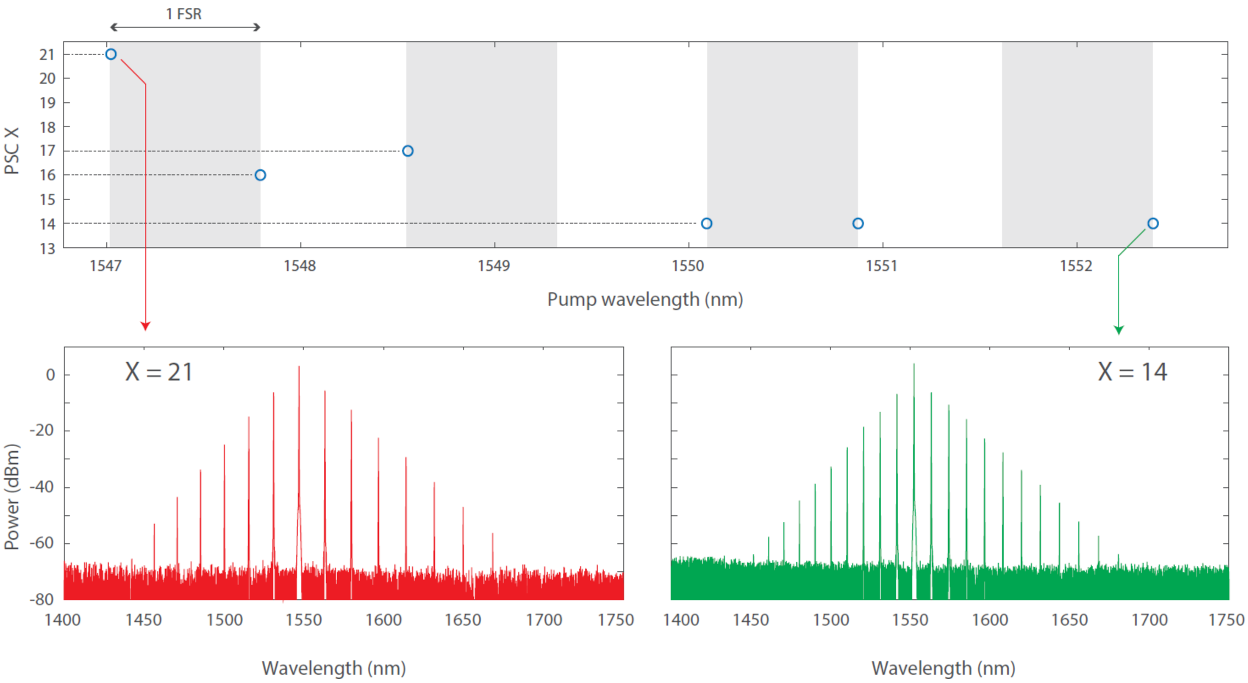


Supplementary Figure 3. **Investigation of the pump wavelength dependence of the maximum soliton number ($X$) of the PSC states generated in the same 100-GHz** $Si_3N_4$ **microresonator.** Top: Wavelength dependence of X in several adjacent resonances. Bottom: two examples of PSC states with $X = 21$ and $X = 14$, generated under the same pump power, but pumping different resonances of the same device.

**Soliton number in PSC states**

The maximum number of the DKS pulses, which can be stabilized in the microresonator is an important parameter defining the number of pulses ($X$) in a PSC state for a given system. However, the derivation of the theoretical framework able to exactly predict this value for a real arbitrary microresonator system is beyond the scope of the current manuscript due to a complex interplay of multiple interaction processes which need to be accounted for together with additional simulations and experiments. Nevertheless, we introduce here several parameters of the system, and phenomenologically explain how they impact the maximum soliton number ($X$) and can provide a good estimation for it.

We start by considering the simplest case of the pure LLE model with the dispersion limited to the second order: $\omega_\mu = \omega_0 + \mu D_1 + 1/2 \cdot \mu^2 D_2$. In such a system, the maximum number of solitons which can stably coexist in the cavity ($N_{max}$) is linked to their duration and is set by the minimum distance at which solitons do not interact with each other [6, 7]: $N_{max} \sim \sqrt{\frac{\kappa}{D_2}}$, where $\kappa$ - is the total cavity decay rate as defined in the first section. From our experience, this number provides a good first-order estimation for the number of DKS pulses forming a PSC state. For example, if we consider 100-GHz $Si_3N_4$ microresonator used in the main manuscript estimated $N_{max} \sim 12$, while the real one is 15 for a given resonance used in the experiments.

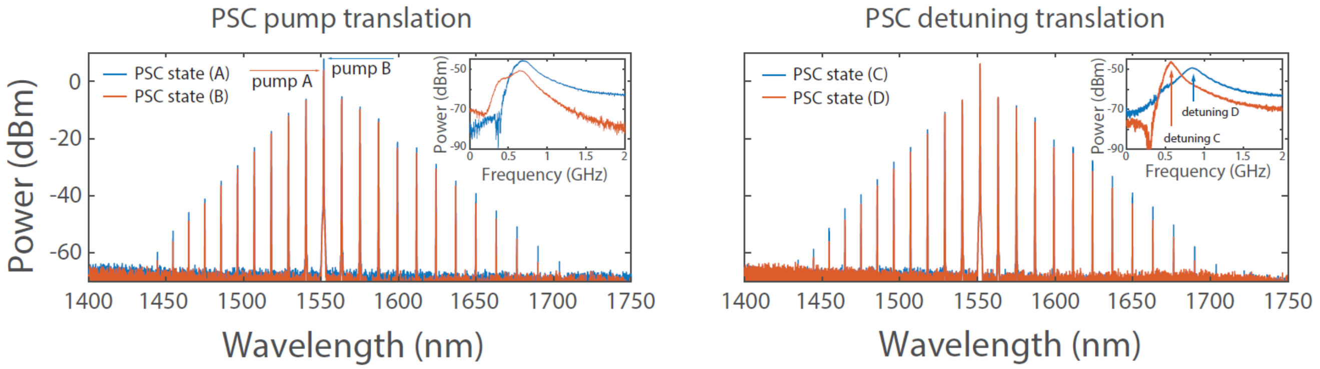


Supplementary Figure 4. **Experimental power and detuning translations of the PSC states.** (Left) Power translation of the PSC states from the pump power A (blue) to pump power B (red), separated by $\sim$ 4dB. Inset shows the VNA probing of the effective detuning in both states [8] to demonstrate that the detuning was maintained. (Right) Detuning translation of the PSC state from the detuning value C (red) to the detuning value D (blue), separated by $\sim$ 0.3 GHz. Inset demonstrates the VNA measurement of the effective detuning in both states.

The next important factor impacting the maximum soliton number available for the given microresonator system is the presence of avoided modal crossings (AMXs). AMXs induce frequency-localized deviations of the DKS optical spectra from the standard $sech^2$-based shape. This results in the formation of the modulated intracavity background from the interference between the pump and the lines comprising such deviations. As was shown earlier [5] and highlighted in the main text of the present manuscript, this AMX-induced background modulation of the DKS state is primarily responsible for the regularization of soliton pulse trains and the formation of soliton crystal states (and particularly PSC) in the microresonator. The modulated background can modify the maximum number of the DKS pulses (established above for the pure LLE model), which are able to coexist in the given microresonator stably, and moreover can lead to the formation of PSC states with different $X$, depending on the position of the AMX with respect to the pumped resonance.

In general, it is not only AMXs that can induce the ordering of the DKS pulses via binding to the modulated background. Similar background modulation can be also created by the soliton-induced dispersive waves as well as other effects, such as Kelly sidebands or birefringence, as recently demonstrated in optical fiber cavities [9].

In the real microresonator system, however, it is still difficult to derive the laws which would be able to *exactly* predict a number of solitons in a PSC state for a given device and pump conditions. One of the primary issues concerns very complex dispersion profiles of real systems, which can include high-order dispersion effects and multiple modal crossings of different strength and locations, which significantly deviate the optical spectrum of the states from the ideal soliton shape. In order to further highlight the complexity of the processes behind the generation of the PSC state with certain $X$, we investigated the wavelength dependency of $X$ for a 100-GHz $Si_3N_4$ microresonator, similar to the one used in the main text of the manuscript (see Supplementary Fig.3). Since the system does not have prominent modal crossings, or dispersive waves, and in principle can be described with the dispersion terms limited to

the second order, one can expect that $X$ will be independent on the wavelength. In contrast, as can be seen from the supplementary figure 3, the number of pulses forming the PSC state changes with wavelength in rather unpredictable manner, which does not allow to derive any reasonable pattern and reveal the full combination of physical processes defining these numbers.

Despite such low predictability of the number $X$ for the PSC state, we still consider the PSC variability available for a single device to be an important advantage, which provides access to coherent soliton combs consisting of pure supermodes with variable spacing and power-per-comb line, just by tuning the pump frequency over several FSR.

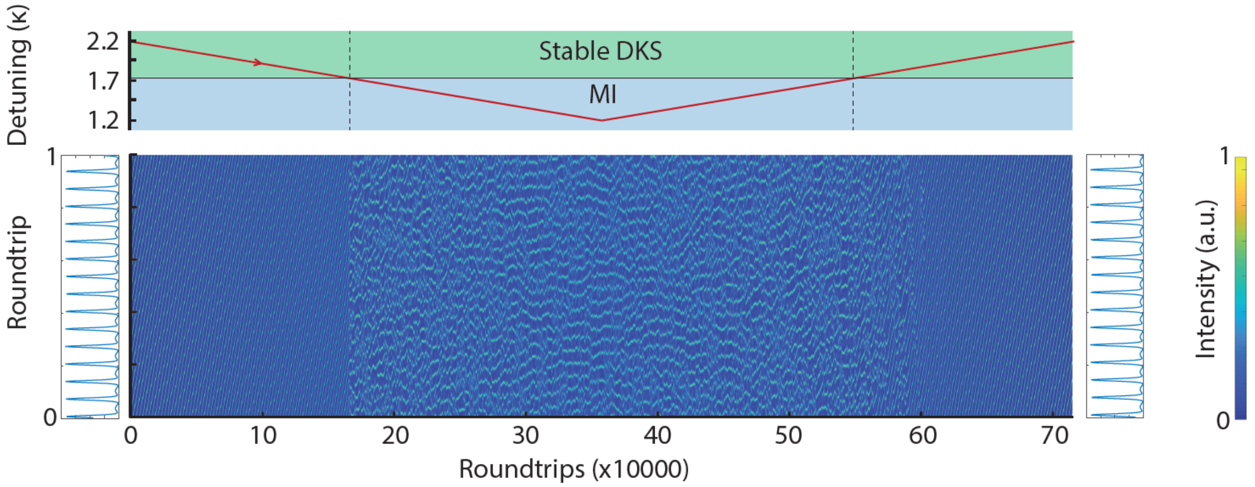


Supplementary Figure 5. **PSC melting and recrystallization** Simulations of the temporal evolution of the intracavity power in a 100-GHz $Si_3N_4$ microresonator from its initial state (left) to its final state (right), while the detuning is changed to move the system to the region of MI and back. Top part of the figure shows the evolution of the detuning.

**PSC state translations**

The power and detuning translations of the PSC states, which were reported in the main text of the present manuscript, are key manipulations which we use to investigate the complex stability chart of these states. Here we would like to experimentally demonstrate that PSC state are indeed able to sustain quite significant translations in power and detuning. Supplementary figure 4 shows two translations (one - in pump power, and one in effective detuning) of the same PSC state generated in the 100-GHz $Si_3N_4$ microresonator of the main manuscript. From the optical spectra we can see that the structure of the PSC state is maintained in both translations. Despite some slight changes in the invidual powers of comb lines due to the increased pump power or change in the efective detuning (which is natural for all DKS states), the system has maintained the number of pulses and exceptional level of their ordering.

**PSC and other regularized multiple-soliton states**

In this section we highlight certain differences between the PSC states presented in our manuscript and other multiple-soliton states, which exhibit soliton ordering and are able to form symmetric states with less number of pulses similar to the PSC (regularized multiple-soliton states). [10–12]. Despite the fact that both states represent very similar formations of ordered ensembles of DKS pulses, there are two distinctions which we would like to emphasize. The first one concerns the deterministic access to such states. In contrast to the regularized multiple-soliton states[10–12] the PSC states demonstrated in our work contain maximum number of DKS pulses available for a given system under given pump conditions. Unlike PSC states, all regularized multiple-soliton states were reported to be obtained stochastically, whether they have resulted from the forward tuning technique [7] or obtained in backward switching [8, 12]. Indeed, one can obtain regularized multiple-soliton states with the number of solitons less than the maximum for a given system only through the interaction with chaotic regions (STC and more importantly TC). We can give the following example: consider an ideal microresonator with a single-mode AMX located 12 FSR away from the pumped resonance and having dispersion profile which stabilizes the same maximum number of pulses in the cavity. When the DKS state is formed, the AMX-induced modulation on the intracavity background creates 12 potential sites for the binding of DKS pulses, which in turn can support the formation of soliton states with 2, 3, 4, 6 or 12 equispaced pulses. While the generation of the PSC state with $X$ = 12 will be deterministic in such a system by

following all the procedures presented in our manuscript, all the other states (with 2, 3, 4 or 6 equispaced solitons) have to be generated by involving the TC regime, because one needs to clear the cavity of excessive pulses created by MI. Since the impact of the TC is unpredictable in terms of the order of soliton elimination either for the forward or backward tuning approaches - the generation of such regularized multiple-soliton states with the soliton number smaller than the maximum number of soliton pulses available for such system can not be done deterministically. Such unpredictability in the generation of such states represents critical limiting factor for their applications, but is fortunately absent for PSC states. The second difference between PSC states and regularized multiple-soliton states with a lower number of solitons, which can be stochastically obtained in the same system, is more subtle and concerns their stability diagram. It was already partially explained in the second section of the present supplementary information. Due to the close packing of the soliton pulses in the PSC, the adjacent DKS pulses tend to interact more strongly when entering the STC region, and can lead to DKS collisions and state switching. This process results in the lowering of the boundary of the TC region for PSC states, which we observed to be at around $f \sim 4$ in dimensionless power amplitude. However, for lower soliton number, the state will sustain the STC region, and thus the region of TC will start for such regularized multiple-soliton states at higher pump powers, closer to $f \sim 5$.

**Simulations of soliton crystal melting and recrystallization**

In order to clearly demonstrate that the microresonator system seeded with a PSC state can indeed experience the excursion to the region of chaotic modiulation stability (melting) and then return back to the initial PSC state (recrystallization), we reproduced the experimentally observed behaviour in simulations.

We choose the pump power of 0.20 W (below the region of spatiotemporal chaos) and launched the initial PSC state (see Supplementary Fig.4, left), then the detuning was changed linearly from 440 MHz to 240 MHz and back in order to bring the system in the MI state and then back to the regime of stable DKS. Recording the temporal evolution of the intracavity power, one can see that the initially seeded PSC state sustains the detuning change, while the system stays within stable DKS region. Sudden change in the behaviour happens when the system enters the MI region – the PSC state loses the long-range ordering, and the system behaviour changes to chaotic [13], in which the transient optical pulses experience multiple interactions, decays and stochastic short-timescale drifts. Once the system is brought back to the stable DKS regime, the transient pulses suddenly reorganize themselves back into the PSC state similar to the initial one.

**Supplementary References**


[1] Leo, F., Gelens, L., Emplit, P., Haelterman, M. & Coen, S. Dynamics of one-dimensional Kerr cavity solitons. *Optics express* **21**, 9180–91 (2013). URL http://www.opticsexpress.org/abstract.cfm?URI=oe-21-7-9180.

[2] Wang, W. *et al.* Robust soliton crystals in a thermally controlled microresonator. *Optics letters* **43**, 2002–2005 (2018). URL https://doi.org/10.1364/OL.43.002002.

[3] Lucas, E., Karpov, M., Guo, H., Gorodetsky, M. & Kippenberg, T. Breathing dissipative solitons in optical microresonators. *Nature communications* **8**, 736 (2017). URL https://doi.org/10.1038/s41467-017-00719-w.

[4] Lu, Z. *et al.* Deterministic generation and switching of dissipative kerr soliton in a thermally controlled micro-resonator. *arXiv preprint arXiv:1810.04983* (2018).

[5] Cole, D. C., Lamb, E. S., Del'Haye, P., Diddams, S. A. & Papp, S. B. Soliton crystals in kerr resonators. *Nature Photonics* **11**, 671 (2017). URL https://doi.org/10.1038/s41566-017-0009-z.

[6] Wabnitz, S. Suppression of interactions in a phase-locked soliton optical memory. *Opt. Lett.* **18**, 601–603 (1993). URL http://ol.osa.org/abstract.cfm?URI=ol-18-8-601.

[7] Herr, T. *et al.* Temporal solitons in optical microresonators. *Nat. Photon.* **8**, 145–152 (2014). URL http://dx.doi.org/10.1038/nphoton.2013.343.

[8] Guo, H. *et al.* Universal dynamics and deterministic switching of dissipative kerr solitons in optical microresonators. *Nat. Physics* **13**, 94–102 (2017). URL https://doi.org/10.1038/nphys3893.

[9] Wang, Y. *et al.* Universal mechanism for the binding of temporal cavity solitons. *Optica* **4**, 855–863 (2017). URL https://doi.org/10.1364/OPTICA.4.000855.

[10] Brasch, V. *et al.* Photonic chip–based optical frequency comb using soliton Cherenkov radiation. *Science* **351**, 357–360 (2016). URL http://dx.doi.org/10.1126/science.aad4811.

[11] Webb, K. E., Erkintalo, M., Coen, S. & Murdoch, S. G. Experimental observation of coherent cavity soliton frequency combs in silica microspheres. *Optics Letters* **41**, 4613–4616 (2016).

[12] Joshi, C. *et al.* Thermally controlled comb generation and soliton modelocking in microresonators. *Opt. Lett.* **41**, 2565–2568 (2016). URL http://ol.osa.org/abstract.cfm?URI=ol-41-11-2565.

[13] Anderson, M., Leo, F., Coen, S., Erkintalo, M. & Murdoch, S. G. Observations of spatiotemporal instabilities of temporal cavity solitons. *Optica* **3**, 1071–1074 (2016). URL http://www.osapublishing.org/optica/abstract.cfm?URI=

optica-3-10-1071.
